# Supplementary material for: Hot Hydride Superconductivity above 550 K
Source: arXiv:2006.03004 source file (2020-06-04)
Supplement: Supplementary file 1 [file Supplementary_information_Grockowiak_20200525.pdf]

# Supplementary information

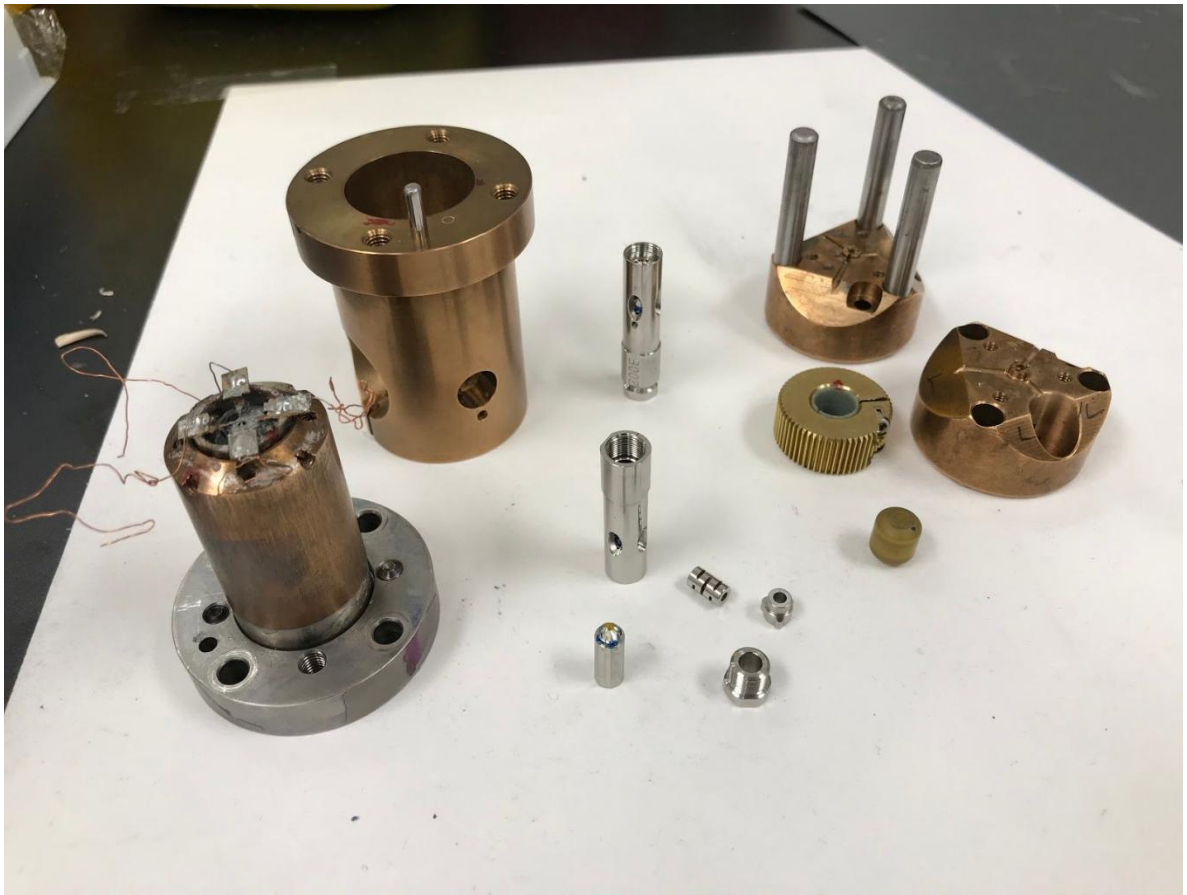

**Figure S1:** Pressure cells used and proposed for superhydrides synthesis: left, UIC Mao-Bell DAC; center, DACs used for this study (B002 is assembled in the background with the parts of B003 in the foreground (The piston diameter is 5.38. mm, total weight is 12.88 g); right, in foreground, plastic DAC that is typically used for our pulsed field work (with ancillary parts to assist in loading shown in the background). Interestingly, the load necessary to generate the 1 to 2 Mbar pressures for synthesis of the hydrides is quite small which opens up the possibility of using this DAC \cite{Graf_2011} for these studies. It can be rotated at He-3 temperatures in pulsed fields and has no metal parts other than the electrical leads and, in this case, the sample.

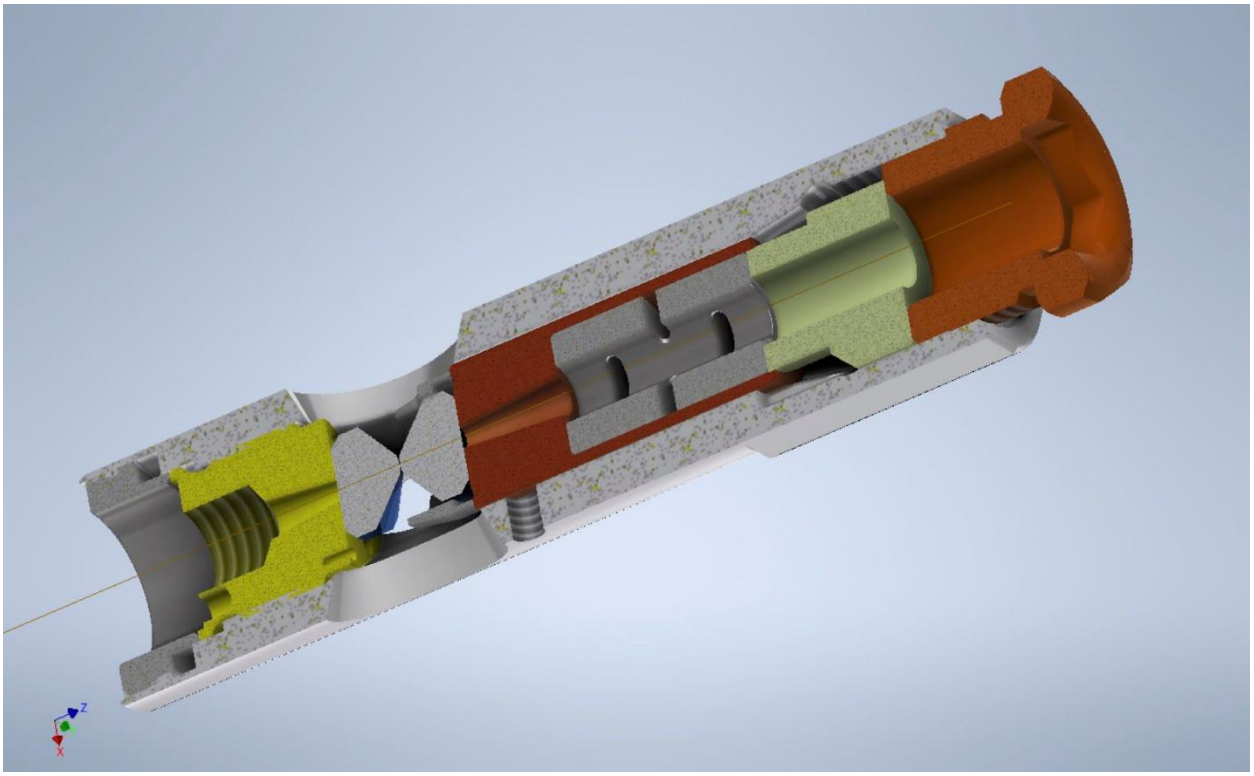

**Fig S2** Model of the DAC used in these studies. All of the metal parts of the DAC are made from Pascalloy, but the parts are shown in different colors for clarity. The anvil with electrodes (external leads not shown) is attached to the endcap to the left in this image while the anvil on the right is attached to a piston that is spring loaded. Both anvils are secured using Stycast 2850FT blue/24 LV epoxy. The gasket and gasket table are electrically isolated from the rest of the DAC. The light green piece has three tabs that register with mating half cylinders in the body of the DAC to prevent the load nut (brown) to the far right from spinning the piston anvil when the load is increased so as to prevent damage to the sample or anvils.

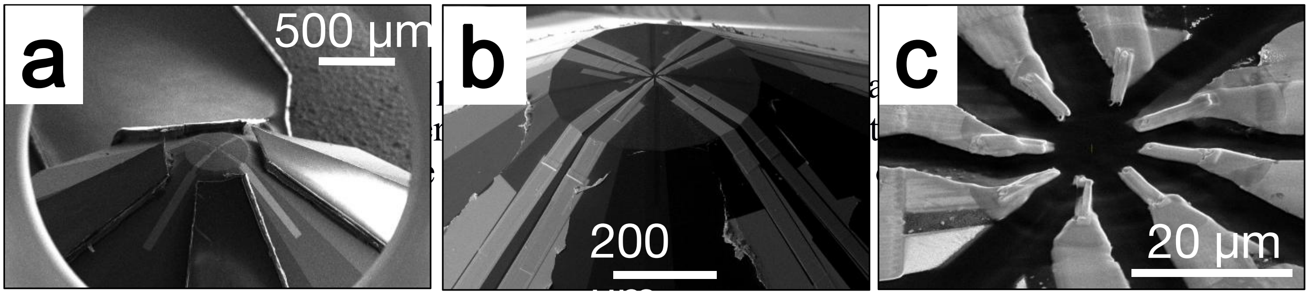


**Fig S3** Images from the FIB processing "a" shows the Kapton tape used to mask the stone prior to gold sputtering; "b" is the resulting AuPt overlay tha has been defined with Ga, and "c" is an image of eight electrodes with tabs on top of the culet.

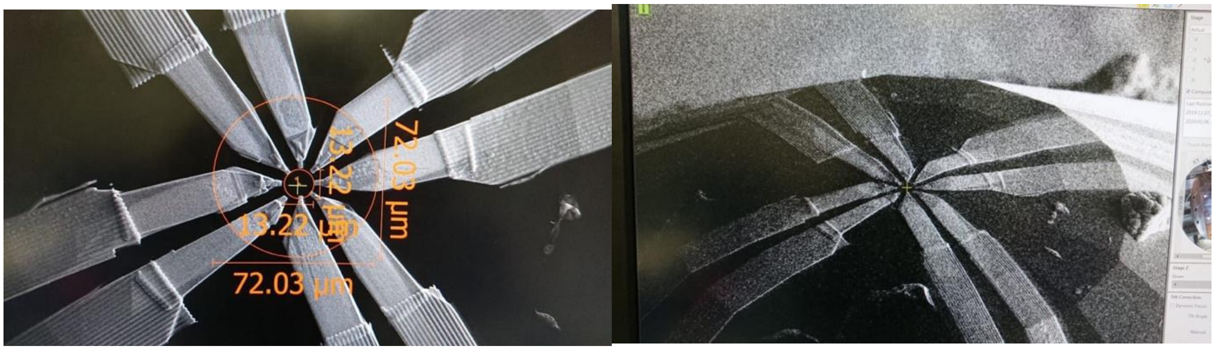


**Fig S4** Two images of the FIB electrode fabrication on the anvil. Left: A closeup of the Pt/Au/Pt electrodes is shown in which an overlay defines the edge of the 72 µm culet. The small tabs grown from the main electrodes encompass a 13 µm circle. Right: Image shows the electrodes draped over the bevels and extending down the pavilion.

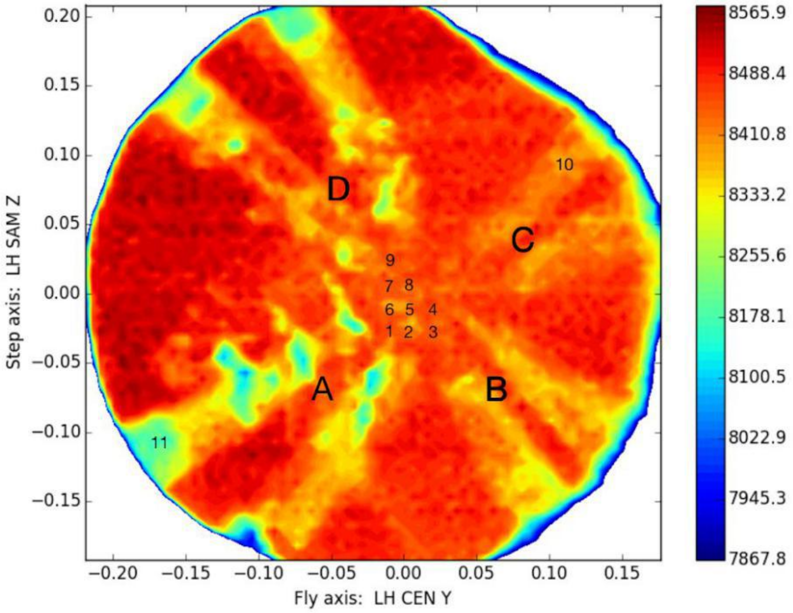


**Figure S5** : Image through the DAC B002 prior to the synthesis using X-ray transmission detected by a photodiode. The color scale indicates the x-ray transmission intensity, with red showing more transmission. The Pt/Au electrodes appear clearly in yellow. The letters indicate electrode pairs, the spots 1 to 9 indicate location of laser heating and subsequent XRD, 10 and 11 XRD spots were for background subtraction. The laser was rastered in a 10 µm x 10 µm grid between spots 1 to 9, starting at 20% (41.5 W) of max laser power and then increased in 5% steps up to 70% laser power, or until coupling between laser and sample is observed to produce a temperature in the range of 1200 K. Coupling was characterized by a flash in the visual image of the sample and the temperature measured at the sample by a black body fit of the signal. The laser was pulsed 4 to 5 times at each spot, at which point a diffraction pattern was obtained. Spots 10 and 11 were diffraction patterns taken only to obtain info on the gasket and electrodes for the purpose of background subtraction. 20 KeV X-rays did not show any scattering, but this is most likely due to the DAC's small 11.5° upstream angle and almost equally small 14° downstream angle.

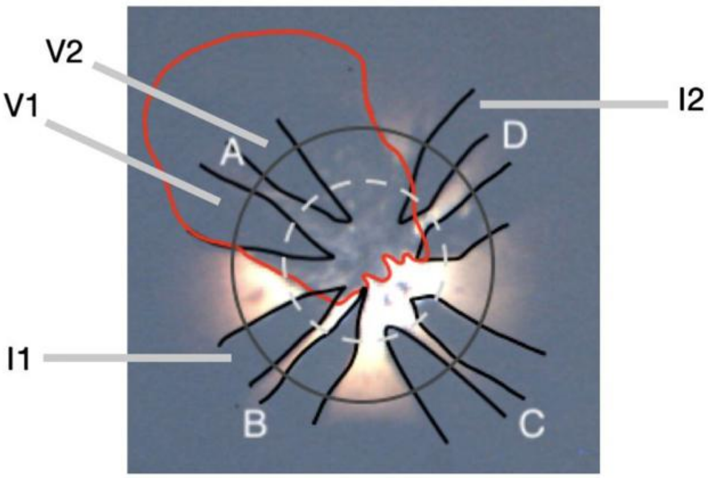
V2
V1
A
D
I2
I1
B
C

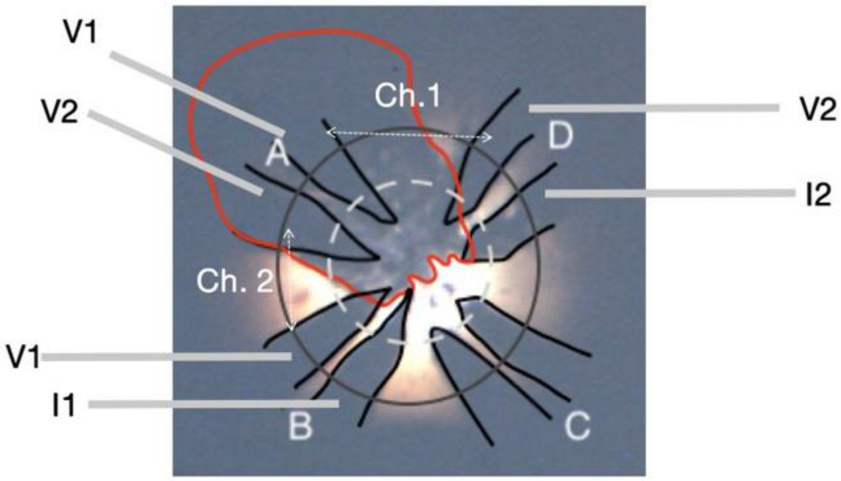
V1
V2
Ch.1
A
D
V2
I2
Ch. 2
V1
I1
B
C

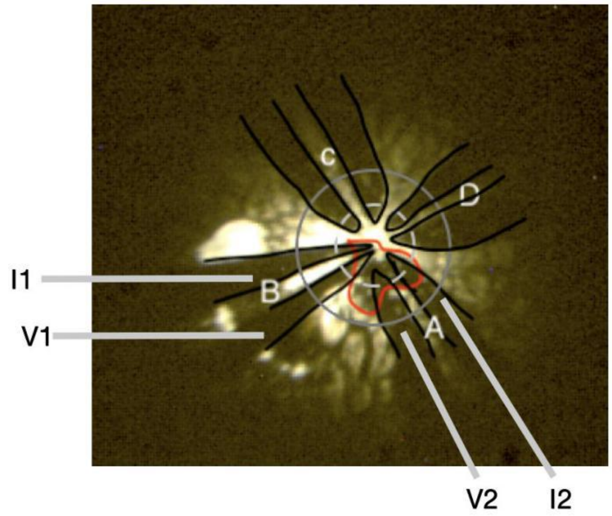


**Figure S6**: top: first electrode configurations for B002 used for the 294 K $T_c$ measurement in the PPMS; top right, Channel 1 (Ch1) of the second electrode configuration was used for subsequent runs in the PPMS. Ch1 and Ch2 were also measured in the 41.5 T resistive magnet. Bottom : electrodes configuration for B003.

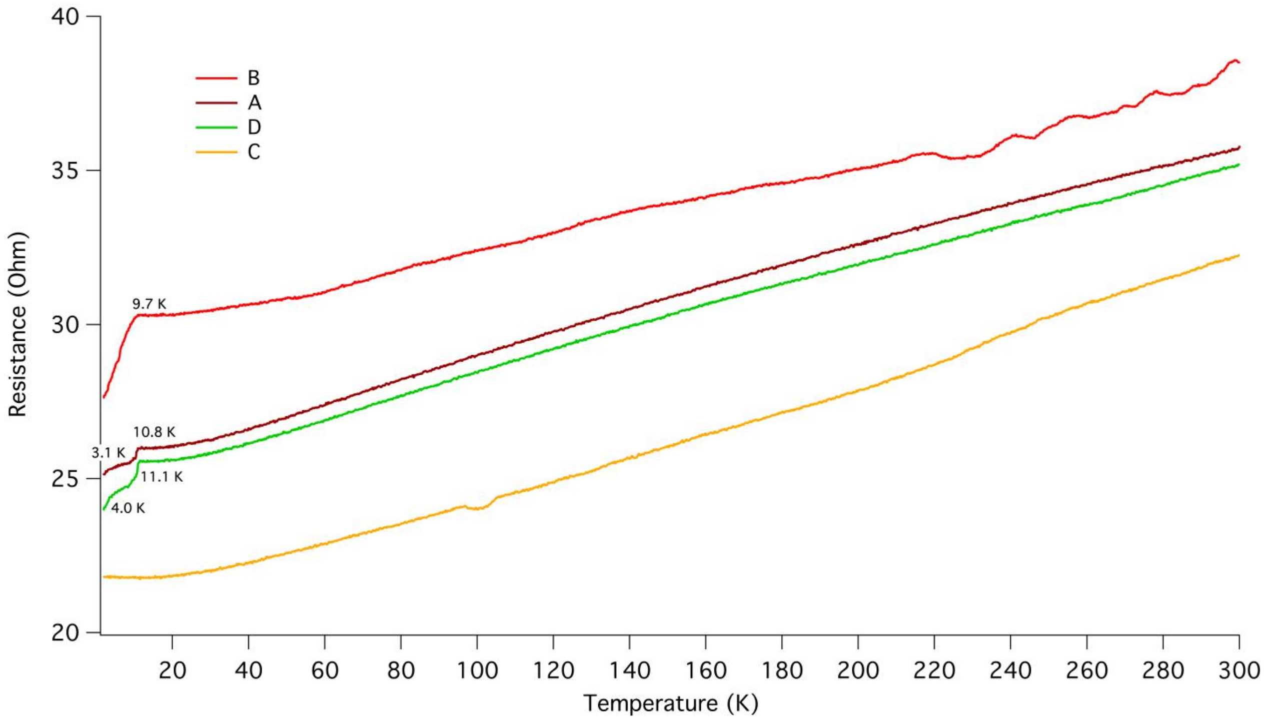


**Figure S7 Comparison of various pseudo 4-probe measurements for B002 taken after the 580 K temperature excursion** Electrode pair C is the open pair that only measures the MP35N gasket and the short between the leads caused by residual gold from the sputtering. A, B and C exhibit superconducting transitions below 15 K with the slope of all curves in the normal state being comparable. The biggest contribution to the background at temperatures higher than 100 K is from the MP35N gasket (see Fig. S8). Electrode pair B shows one strong superconducting transition at 9.7 K which is also observed at 10.8 K in A, and 11.1 K in D. We rule out a superconducting transition of elemental La as those $T_c$'s would indicate a pressure well below 1 GPa \cite{Chen_2019}. These transitions are more likely from a lower stoichiometry La superhydride, with the difference in $T_c$ between the electrode pairs being due to compositional variations following an inhomogeneous synthesis, and/or a gradient of pressure across the culet. It is also possible that the platinum electrode reacted with the hydrogen to form a hydride \cite{Scheler_2011}. We attribute the transitions around 3 to 4 K to elemental La captured between the bevels, although the optical image of B002 does not show any La between the bevels of electrodes D. If it is due to elemental La, it is more likely unreacted La on the culet as the value of $T_c$ would indicate pressures of the order of 110 to 130 GPa. \cite{Chen_2019}

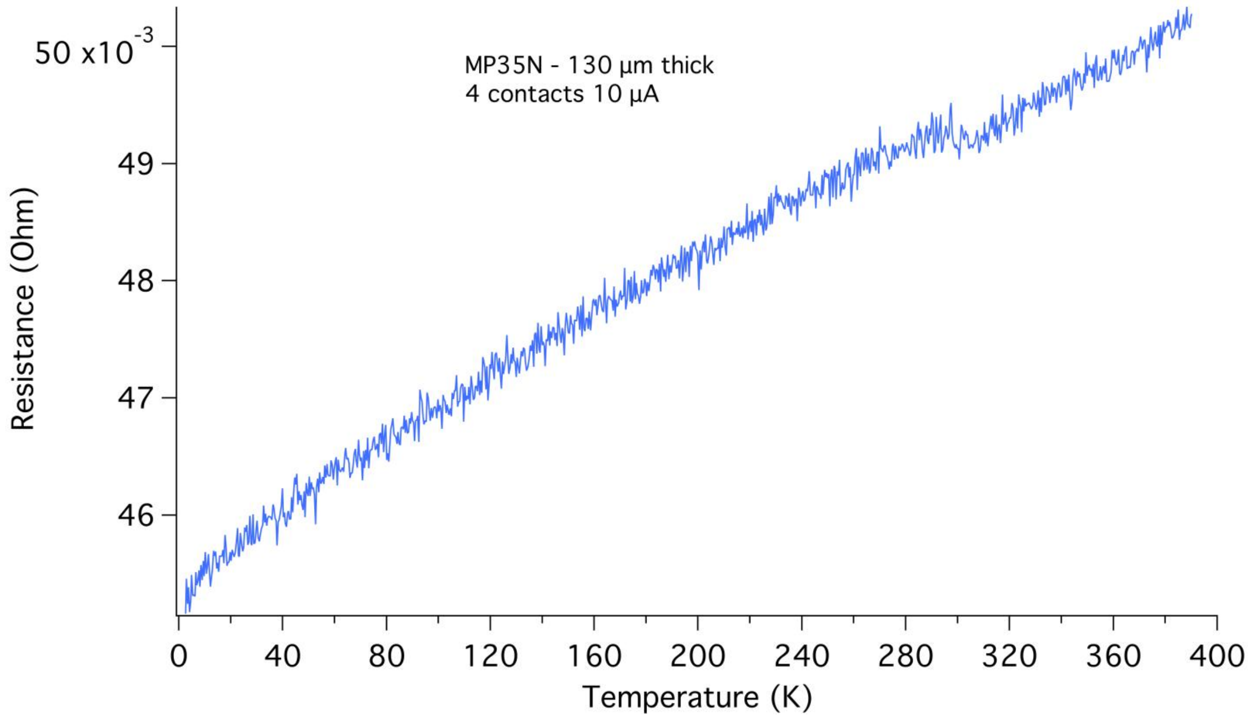


**Figure S8**: To rule out any transition originating from the gasket and to determine the background contributed by the short to the gasket, a 4-probe electrical transport measurement at 0 T of a 135 µm strip of MP35N was made in the PPMS (this is the same material as used for the gasket). The kink around 300 K is due to a change in the temperature sensor used by the PPMS for the higher temperature range. No transitions were observed for MP35N.

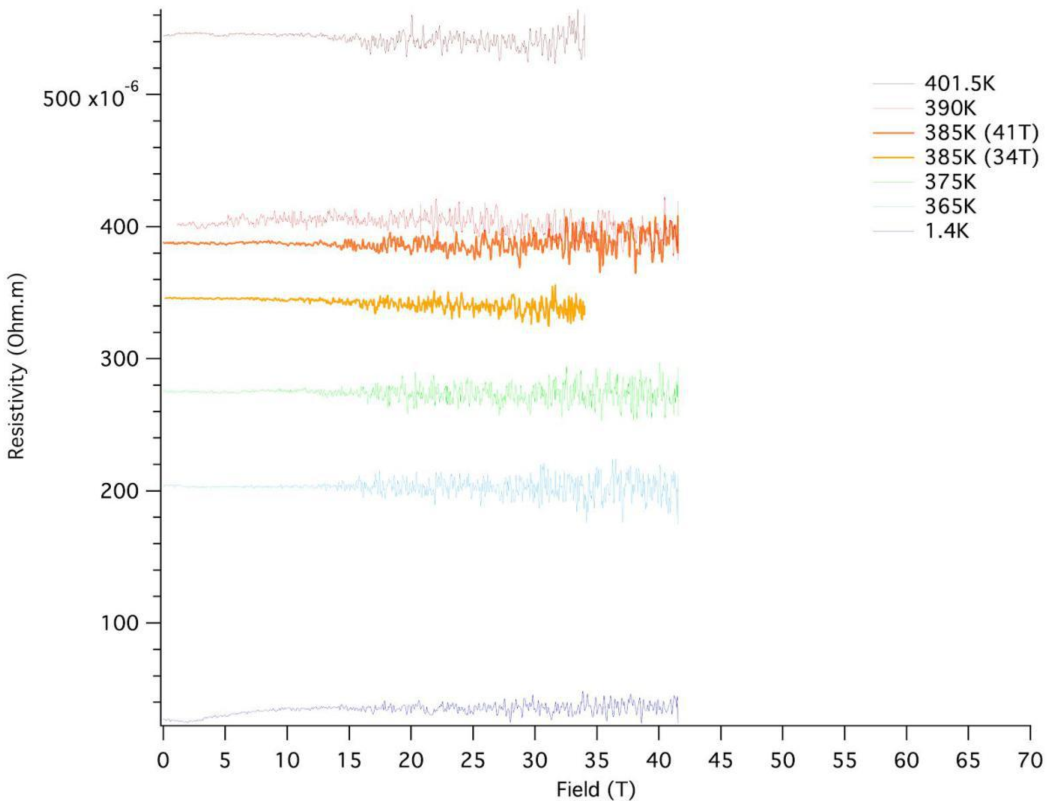


**Fig S9** Magnetoresistance of B002 (configuration 2) at fixed temperatures showing noise level and nothing visible in the signal to indicate $H_c$.

## Journal of peak temperatures

To better establish the thermal pattern that led to the observed superconducting transitions, we provide a table of local maximum temperatures and the time spent at each one. We define a local maximum as the highest temperature reached before it is reduced by more than 10 K and the time as the continuous interval during which the temperature remained within 10 degrees of the stated peak, both before and after reaching that peak.

| Datetime | Peak temperature (K) | Minutes within 10 K of peak |
|---|---|---|
| 3/20/20 5:44 PM | 381.7 | 22 |
| 3/20/20 8:02 PM | 380.7 | 182 |
| 3/20/20 11:57 PM | 390.1 | 26 |
| 3/21/20 1:30 AM | 389.9 | 23 |
| 3/23/20 3:12 AM | 385.4 | 87 |
| 3/23/20 2:43 PM | 391.2 | 23 |
| 3/23/20 4:24 PM | 392.3 | 83 |
| 3/23/20 7:31 PM | 396.2 | 19 |
| 3/23/20 10:52 PM | 391.2 | 19 |
| 3/24/20 8:02 AM | 385.1 | 295 |
| 3/24/20 12:18 PM | 385.1 | 69 |
| 3/24/20 2:19 PM | 289 | 10 |
| 3/24/20 4:57 PM | 27.1 | 23 |
| 3/24/20 9:40 PM | 385.6 | 57 |
| 3/25/20 12:40 AM | 404 | 13 |
| 3/25/20 12:59 AM | 402.2 | 42 |
| 3/25/20 3:50 AM | 400.2 | 62 |
| 3/25/20 9:05 AM | 390.1 | 159 |
| 3/25/20 11:41 AM | 406.4 | 123 |
| 3/25/20 2:03 PM | 411.1 | 462 |
| 3/26/20 12:37 AM | 410.3 | 89 |
| 3/26/20 6:51 AM | 405.2 | 121 |
| 3/26/20 12:15 PM | 432.6 | 240 |
| 3/26/20 3:08 PM | 430.7 | 34 |
| 3/26/20 7:10 PM | 445.4 | 70 |
| 3/27/20 8:57 AM | 493 | 11 |
| 3/27/20 9:18 AM | 500.5 | 52 |
| 3/27/20 1:46 PM | 500.2 | 149 |

| | | |
|---|---|---|
| 3/27/20 8:54 PM | 503 | 54 |
| 3/27/20 11:09 PM | 503.1 | 72 |
| 3/28/20 3:35 PM | 530.7 | 38 |
| 3/29/20 3:12 PM | 530 | 304 |
| 3/30/20 2:21 PM | 530.1 | 278 |
| 3/30/20 5:19 PM | 530.8 | 52 |
| 3/30/20 7:48 PM | 525.4 | 58 |
| 3/30/20 11:10 PM | 525.4 | 60 |
| 3/31/20 2:05 AM | 525.4 | 69 |
| 3/31/20 5:54 AM | 525.7 | 221 |
| 3/31/20 11:52 AM | 525.7 | 58 |
| 3/31/20 2:43 PM | 525.6 | 112 |
| 3/31/20 5:21 PM | 480.9 | 14 |
| 3/31/20 8:04 PM | 527.3 | 48 |
| 3/31/20 10:43 PM | 525.4 | 60 |
| 4/1/20 1:39 AM | 525.4 | 69 |
| 4/1/20 11:35 AM | 320.3 | 128 |
| 4/2/20 12:52 PM | 48.6 | 304 |
| 4/3/20 3:43 AM | 524.8 | 45 |
| 4/3/20 10:19 AM | 580 | 39 |

## Thermometer recalibration including the magnetoresistance

Contrary to the raw data obtained in the 41.5 T resistive magnet, the temperatures measured in the PPMS are internally corrected for field effects. In the 41.5 T resistive magnet setup, the temperature was measured via a Pt-100 sensor placed inside the DAC's body, against the piston anvil. The resistance of this sensor is measured by a Lakeshore 370, and converted to a temperature by using a calibration curve provided by the manufacturer at zero magnetic field and up to 1200 K. As our results are resistance traces at fixed magnetic field, we had to take into account the magnetoresistance of the Pt sensor to recalculate the temperature. Two independent approaches presented below yielded the exact same correction.

### Extrapolation of low field and low temperature magnetoresistance data.

The Pt sensor magnetoresistance (MR) was measured between 0 and 16 T in the PPMS at several temperatures between 240 and 390 K. The MR was fitted at each temperature by a linear and a quadratic fit between 2 and 16 T. The temperature evolution of the coefficients of those fits was then fitted again with a linear and a quadratic fit. Those four fits generated were then extrapolated to 600 K and 41.5 T using the 0 T calibration curve, and used to recalculate the temperature of the high field curves. Details available upon request.

### AI approach

We bootstrapped this calculation by observing that at thermal equilibrium, the heater power and temperature are both stable. Due to the large thermal mass of the cell, it took about 100 seconds for the thermometer (and thermally coupled sample) to rise after adjusting the heater power. After that, additional slower factors made open loop stabilization an impossible task, particularly under time and magnet energy budget constraints. Controlled temperature ramps would have been impossible as well. Instead, we allowed the temperature controller to maintain the provided setpoint or ramp function while the platinum thermometer resistance increased upon increasing field. The controller reduced heater output to match the measured value to the setpoint. Therefore, the actual temperature of the thermometer was less than the setpoint and measured values.

The actual temperature must be obtained by examining the power output of the heater. The thermal lag between the heater and thermometer (sample) complicates

matters, as it is an unknown function of time and temperature. To determine this function, we chose 22 sets of continuous temperature data that began from thermal equilibrium. In each case, we took the longest possible set of data, even when that meant concatenating data files together into a quasi-continuously recorded stream, after accounting for the short gap between files.

There are two coupled problems to solve here. One is the equilibrium response curve between the heater and the thermometer, which is both nonlinear and also includes a contribution from the temperature of the surrounding cryogenic space. The other is the time-dependent portion. In our first attempt, we tried to solve the time-dependent portion by fitting poles and zeros to form a rational transfer function in the $s=j\omega$ domain, then applying the filter from an equilibrium point, but that left no mechanism by which to determine and adjust for nonlinearities in the overall heater-thermometer curve.

Instead, we employed a Deep Learning (DL) technique using fast.ai[1] as an interface to PyTorch [2] to model the entire nonlinear system. Deep Learning, colloquially called Artificial Intelligence, propagates inputs through layers of variables more numerous than the inputs themselves. Each layer includes a nonlinear function and a linear matrix operation. Coefficients are optimized iteratively on a portion of the data through a process called "training." Then, the model is compared to a non-intersecting portion of the data, called "validation." Input parameters were the heater output (0-100%) and VTI sample space temperature (242-319 K) Since a rational transfer function is not amenable to this technique, we provided the DL tool 40 taps of past values in both parameters with which it could form a sort of FIR filter. Tap delay ranged from 5 to 1310 seconds, which covers most of the response of the system.

Since the DL tool was solving two problems at once, we found that it simultaneously underfit the temporal problem while overfitting the equilibrium problem. Our result is very much dependent on an accurate, monotonic equilibrium response, so we fit Chebyshev polynomials to the equilibrium result over the (VTI temperature, heater %) input space, then augmented the original input with that smoothed dataset. We ran the DL tool a second time to refine the temporal behavior while retaining the smooth equilibrium one. The resulting model could predict the temperature of the sample from the values and history of the VTI environment and the sample heater.

We applied the model to 14 upsweep magnet ramps of varying speeds and limits. Some included pauses at intermediate fields to verify the health of the magnet as

well. During these pauses, we can observe that the slope of measured temperature vs. time is the same as the overall slope of the predicted temperature vs. time, thus verifying the accuracy of the DL model. Predicted temperatures from the model were adjusted up or down so they began at the zero-field indicated thermometer temperature. We then subtracted the thermometer data vs. time from the predicted temperature vs. time, and plotted this "correction" trace as a function of field. The name correction is used because it may be added to magnetoresistive thermometer data to recover the actual temperature.

Observing (without surprise) that the correction traces seemed to be quadratic in field, we fit them with single-term $k_iB^2$ polynomials. Data at similar temperature ranges were grouped together for fitting, although we tried this several ways with no effect on the result. Finally, we considered the $k_i$ polynomial coefficients as a function of temperature. Since magnetoresistance generally falls to zero at very large temperatures, we plotted them in inverse temperature and observed empirically quadratic behavior. The correction function (valid within 0.2 K tolerance for 300 <= $T$ <= 530 kelvin and 0 <= $B$ <= 41.5 tesla) for our Lakeshore Pt-100 platinum thermometer is – 180 $B^2/T^2$.

[1] Jeremy Howard et al. fastai. https://github.com/fastai/fastai, 2018.

[2] Adam Paszke, Sam Gross, Francisco Massa, Adam Lerer, James Bradbury, Gregory Chanan, Trevor Killeen, Zeming Lin, Natalia Gimelshein, Luca Antiga, Alban Desmaison, Andreas Kopf, Edward Yang, Zachary DeVito, Martin Raison, Alykhan Tejani, Sasank Chilamkurthy, Benoit Steiner, Lu Fang, Junjie Bai, and Soumith Chintala. Pytorch: An imperative style, high-performance deep learning library. In H. Wallach, H. Larochelle, A. Beygelzimer, F. dAlch́e-Buc, E. Fox, and R. Garnett, editors, Advances in Neural Information Processing Systems 32, pages 8024–8035. Curran Associates, Inc., 2019.

The first magnetoresistance estimation yielded 4 possible corrections, the artificial intelligence approach gave a quadratic correction with field. We plot below the second quadratic fit given by the first approach (labeled ADG), against the results given by the AI approach (labeled WAC). The results are quasi-identical and validate the correction.

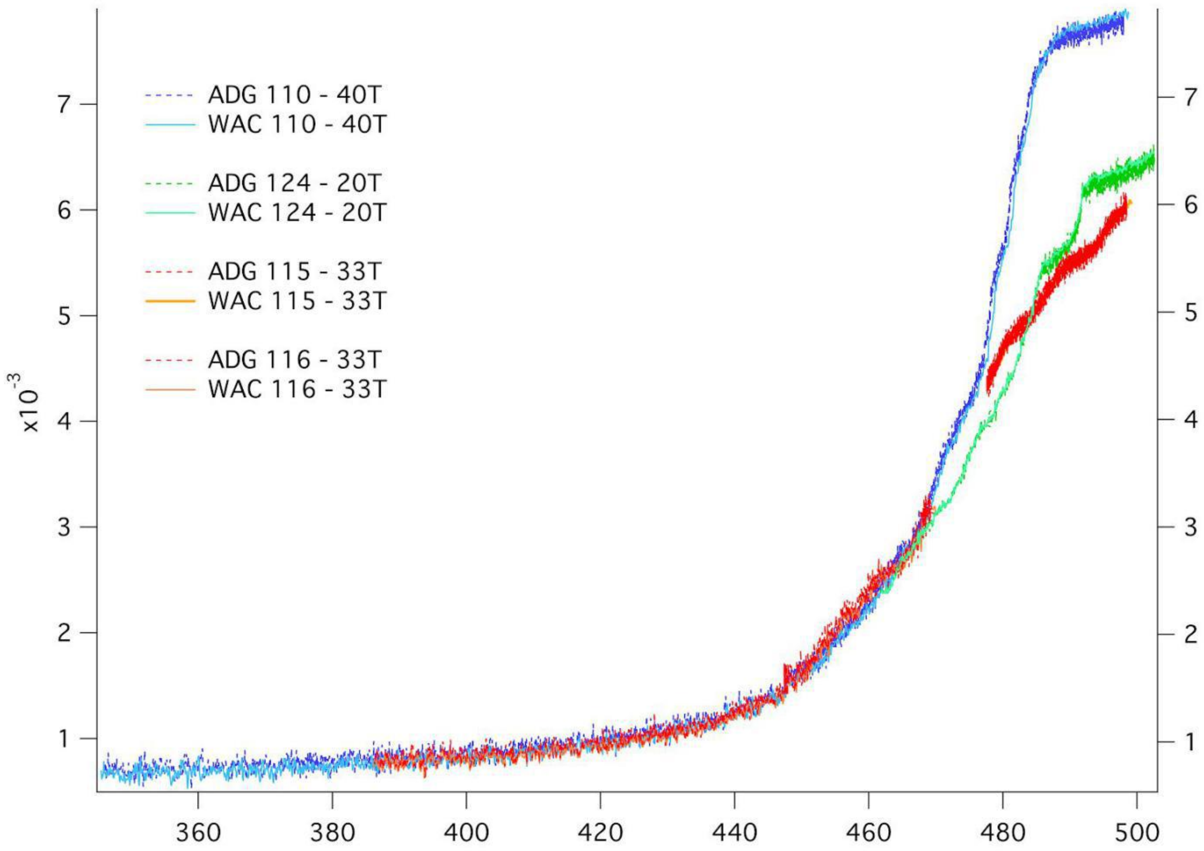


# References :

@Article{Graf2011,
author = {D. E. Graf and R. L. Stillwell and K. M. Purcell and S. W. Tozer},
journal = {High Pressure Research},
title = {Nonmetallic gasket and miniature plastic turnbuckle diamond anvil cell for pulsed magnetic field studies at cryogenic temperatures},
year = {2011},
month = {dec},
number = {4},
pages = {533--543},
volume = {31},
doi = {10.1080/08957959.2011.633909},
publisher = {Informa {UK} Limited},
}

@Article{Chen2019,
author = {Wuhao Chen and Dmitrii V. Semenok and Ivan A. Troyan and Anna G. Ivanova and Xiaoli Huang and Artem R. Oganov and Tian Cui},
title = {{Superconductivity and Equation of State of Distorted FCC-Lanthanum above Megabar Pressures}},

date = {2019-03-06},
eprint = {1903.02194v2},
eprintclass = {cond-mat.supr-con},
eprinttype = {arXiv},
file = {:http\://arxiv.org/pdf/1903.02194v2:PDF},
keywords = {cond-mat.supr-con},
}

@Article{Scheler_2011,
author = {Thomas Scheler and Olga Degtyareva and Miriam Marqu{\'{e}}s and Christophe L. Guillaume and John E. Proctor and Shaun Evans and Eugene Gregoryanz},
journal = {Physical Review B},
title = {Synthesis and properties of platinum hydride},
year = {2011},
month = {jun},
number = {21},
volume = {83},
doi = {10.1103/physrevb.83.214106},
publisher = {American Physical Society ({APS})},
}
